# Supplementary material for: Probabilistic Model Checking for Complex Cognitive Tasks -- A case study in human-robot interaction
Source: arXiv:1610.09409 source file (2016-10-28)
Supplement: Supplementary file 1 [file InsufficientDataAppendix.tex]

\section{Quasi Non-determinism due to low confidence}
\label{App:InssuficientConfidence}
Notice that this approach only works if we have sufficient confidence the for each combination of distance and angle to the features for each objective and each movement. If this confidence is insufficient, using an stochastic approximation might be way off. 
One possible solution is to compute with confidence-intervals \cite{}. We however noticed that unless the intervals for the given data are very-tight, the resulting intervals for a given movement become almost 0-1. Moreover, such tight intervals are only possible with either low confidence or with a lot of data, the confidence level for the resulting probabilistic distribution becomes even lower. 
Thus, whenever we do not have high confidence in any of the data which made up the movement-values, the result is almost non-deterministic. We support this directly marking such values as low-confident and translating this into a situation where we have one action per movement.

\begin{definition}
	The MDP $\MdpInit$ reflecting the human behaviour starting in $\humaninit$ on a environment $\Env = (\loc, \Feat, \advGoal, \robotGoal)$ using temperature $\temp$ is given by 
	\begin{itemize}
		\item $\MdpStates = \{ (\humanpos, A) | \humanpos = (\humanloc, \humanangle) \in \loc \times \dir, A \subseteq \Feat \}$
		\item $\sinit = (\humaninit, \Feat)$
		\item $\Act = \Feat^3 \cup \humanActs$
		\item

		For $s$ such that $\forall (a, \vec{x}) \in V(s)$ \textbf{ confident } 
		\begin{align*}\pmdp(s, a) = \begin{cases} \{ 
				\eff{{M_i}}(s) \mapsto \softmax_\temp(\vec{x}_i) |~i \in \{1,2,3\}  \} & \text{for }a \in \Feat^3~\\&\text{s.t.} (a,\vec{x}) \in \movementValues \\
 			\bot & else.\end{cases}
 			 \end{align*}
 			 Otherwise: 
 			 \begin{align*}
 				\pmdp(s, a) = \begin{cases}\{ 
				\eff{{a}}(s) \mapsto 1   \} & a \in \humanActs \\
 			\bot & \text{else.}\end{cases}	
 			\end{align*}
	\end{itemize}

\end{definition}
Notice that if we are not confident about any entry of $V(s)$, the adversary can select any movement with probability $1$. By using a probabilistic scheduler, we can emulate any distribution over the movements, which allows us to leave these options out at the cost of allowing probabilistic schedulers. For typical reachability properties on the MDP, these costs are non-existent, as it suffices to check only check deterministic schedulers.
